# Supplementary material for: MSPipe: Efficient Temporal GNN Training via Staleness-Aware Pipeline
Source: arXiv:2402.15113 source file (2024-07-18)
Supplement: Supplementary file 1 [file appendix_additional_experiment.tex]

% \newpage
% \section{Additional Experiments}
% \subsection{Evaluate on more hardware environments}

% We conducted experiments in Sec. 4.3 on different hardware environments, including machines with 4 V100 and 2 P100 GPUs. The results in the Tab. 3 in the supplement shows that our staleness scheduling mechanism achieves the minimal staleness bound without compromising throughput and model accuracy. While it is possible that the optimal staleness bound may differ for throughput and model accuracy, our experiments show that MSPipe performs exceptionally well in various commonly used hardware environments.

% \begin{table}[]
% \centering
% \begin{tabular}{lllllll}
% \toprule
% \textbf{Hardware} & \multicolumn{2}{l}{\textbf{4 $\times$ A100}} & \multicolumn{2}{l}{\textbf{4 $\times$ V100}} & \multicolumn{2}{l}{\textbf{2 $\times$ P100}} \\
% \midrule
% \makecell{Staleness\\bound} & AP(\%) & \makecell{Epoch\\time(s)} & AP(\%) & \makecell{Epoch\\time(s)}& AP(\%) & \makecell{Epoch\\time(s)} \\
% \midrule
% 0(TGL) & 87.2 & 13.1 & 87.8 & 11.42 & 87.4 & 24.56 \\
% \midrule
% 2(minimal) & 86.9 & 6.55 & 86.3 & 7.15 & 85.9 & 17.57 \\
% \midrule
% 4 & 82.4 & 7 & 82.19 & 7.53 & 82.7 & 18.33 \\
% \midrule
% 8 & 81.8 & 7.24 & 82 & 7.97 & 81.5 & 18.9 \\
% \midrule
% 16 & 78.9 & 7.5 & 77.5 & 9.77 & 78 & 19.17 \\
% \midrule
% 32 & 72.63 & 7.79 & 73.21 & 9.91 & 75.25 & 19.21 \\
% \bottomrule
% \end{tabular}
% \caption{Throughput and AP on different staleness bound with different hardware settings. Use the LastFM dataset to train the TGN model.}
% \label{tab:devices}
% \end{table}
