# Supplementary material for: MSPipe: Efficient Temporal GNN Training via Staleness-Aware Pipeline
Source: arXiv:2402.15113 source file (2024-07-18)
Supplement: Supplementary file 3 [file appendix.tex]

\section{Appendix}
